# Supplementary material for: Neural Alignment for Face De-pixelization
Source: arXiv:2009.13856 source file (2020-09-29)
Supplement: Supplementary file 1 [file 07_supp.pdf]

# Neural Alignment for Face De-pixelization Supplementary Material

## 1. Additional qualitative results

### 1.1. Video

A video clip which describes our method with additional qualitative results and comparisons is attached: `FaceDepixVid.mp4`.

### 1.2. HTML

Additional results are shown in GIF form in the attached HTML file:
`AdditionalResults.html`.

## 2. Network architecture

The full architecture of our pipeline is summarized in the tables below, where Table 2 and Table 3 summerize the architectures of the STN and de-pixelization networks, respectively. Both architectures are composed of a series of different blocks. Table 1 specifies the layers contained in each block, where `Conv2D`, `BN`, `RelU` denote a 2D convolution layer, batch normalization and a rectified linear unit, respectively. In addition, $k$, $p$, $C_{in}$, $C_{out}$ denote kernel size, padding size, channel input size and channel output size, respectively. The SkipConnection column in Tables 2 and 3, points to the index of the layer from which the connection originates.

| Name | layers |
|---|---|
| DoubleConv($C_{in}$, $C_{out}$, k, p) | Conv2D($C_{in}$, $C_{out}$, k, p) + BN + ReLU<br>Conv2D($C_{out}$, $C_{out}$, k, p) + BN + ReLU |
| DownBlock($C_{in}$, $C_{out}$, k, p) | MaxPool(2)<br>DoubleConv($C_{in}$, $C_{out}$, k, p) |
| UpBlock($C_{in}$, $C_{out}$, k, p) | BilinearUpsampling($sampling factor = 2$)<br>Concatenation<br>DoubleConv($2 \cdot C_{in}$, $C_{out}$, k, p) |

Table 1. Blocks layers.

| # | Name | $k$ | $p$ | $C_{in}$ | $C_{out}$ | SkipConnection |
|---|---|---|---|---|---|---|
| (1) | DoubleConv 1 | 3 | 1 | 6 | 32 | - |
| (2) | DownBlock 1 | 3 | 1 | 32 | 64 | - |
| (3) | DownBlock 2 | 3 | 1 | 64 | 128 | - |
| (4) | DownBlock 3 | 3 | 1 | 128 | 256 | - |
| (5) | DoubleConv 2 | 3 | 1 | 256 | 256 | - |
| (6) | UpBlock 1 | 3 | 1 | 256 | 128 | (4) |
| (7) | UpBlock 2 | 3 | 1 | 128 | 64 | (3) |
| (8) | UpBlock 3 | 3 | 1 | 64 | 32 | (2) |
| (9) | Conv2D + Tanh | 3 | 1 | 32 | 2 | - |

Table 2. STN U-Net architecture.

| # | Name | $k$ | $p$ | $C_{in}$ | $C_{out}$ | SkipConnection |
|---|---|---|---|---|---|---|
| (1) | DoubleConv 1 | 3 | 1 | 3·#frames | 64 | |
| (2) | DownBlock 1 | 3 | 1 | 64 | 128 | - |
| (3) | DownBlock 2 | 3 | 1 | 128 | 256 | - |
| (4) | DownBlock 3 | 3 | 1 | 256 | 512 | - |
| (5) | DownBlock 4 | 3 | 1 | 512 | 512 | - |
| (6) | UpBlock 1 | 3 | 1 | 512 | 256 | (4) |
| (7) | UpBlock 2 | 3 | 1 | 256 | 128 | (3) |
| (8) | UpBlock 3 | 3 | 1 | 128 | 64 | (2) |
| (9) | UpBlock 3 | 3 | 1 | 64 | 64 | (1) |
| (10) | Conv2D + Tanh | 3 | 1 | 64 | 3 | - |

Table 3. De-Pixelization U-Net architecture.
